# Supplementary material for: Skeleton-based Group Activity Recognition via Spatial-Temporal Panoramic Graph
Source: arXiv:2407.19497 source file (2024-11-29)
Supplement: Supplementary file 2 [file X_suppl.tex]

\Crefname{section}{}{}


\title{Skeleton-based Group Activity Recognition via Spatial-Temporal Panoramic Graph Supplementary Material}

% TODO REVIEW: If the paper title is too long for the running head, you can set
% an abbreviated paper title here. If not, comment out.
\titlerunning{Skeleton-based GAR via Panoramic Graph}

%%%%%%%%% AUTHORS - PLEASE UPDATE
\author{Zhengcen Li\inst{1,2}\orcidlink{0000-0001-9736-7375} \and
Xinle Chang\inst{1} \and
Yueran Li\inst{1} \and
Jingyong Su\inst{1,2}\textsuperscript{(\Letter)}\orcidlink{0000-0003-3216-7027}
} 

% TODO FINAL: Replace with an abbreviated list of authors.
\authorrunning{Li et al.}
% First names are abbreviated in the running head.
% If there are more than two authors, 'et al.' is used.

% TODO FINAL: Replace with your institution list.
\institute{Harbin Institute of Technology, Shenzhen, 518055, China \and
Peng Cheng Laboratory, 518055, China \\
\email{\{lizhengcen, changxinle, liyueran\}@stu.hit.edu.cn} \\
\email{sujingyong@hit.edu.cn}
}

\maketitle

\bigskip
\bigskip

\noindent\vspace{\baselineskip} This appendix is organized as follows: \\
\Cref{sec:supp-a} Details of Keypoint Acquisition \\
\indent\Cref{sec:supp-aa} Pose Estimation and Tracking \\
\indent\Cref{sec:supp-ab} Reassignment Strategy \\
\Cref{sec:supp-b} Data Pre-processing of Multiple Inputs \\
\Cref{sec:supp-c} Detailed Comparison between Keypoint-based Methods \\
\Cref{sec:supp-d} Additional Qualitative Results \\
\Cref{sec:supp-e} Additional Ablation Studies \\ 


\section{Details of Keypoint Acquisition}
\label{sec:supp-a}

\subsection{Pose Estimation and Tracking}
\label{sec:supp-aa}

    We use the pre-trained YOLOv8x-pose model to estimate human skeletons for Volleyball Weakly Supervised and NBA datasets. Our approach follows the official implementation of YOLOv8\footnote{\href{https://docs.ultralytics.com/tasks/pose}{https://docs.ultralytics.com/tasks/pose}}. The YOLOV8x-pose model conforms to the COCO keypoint layout, which represents a person with 17 keypoints: nose, left eye, right eye, left ear, right ear, left shoulder, right shoulder, left elbow, right elbow, left wrist, right wrist, left hip, right hip, left knee, right knee, left ankle and right ankle. Both the Volleyball and NBA datasets are processed with the maximum number of actors in a single frame $M=12$.
    We maintain the original resolution of each video clip when feed into YOLOv8x, as the videos in both Volleyball and NBA datasets have resolutions of $1920\times1080$ and $1280\times720$. For pose tracking, we ultilize the integrated BoT-SORT~\cite{aharon2022botsort} tracker with default YOLO tracker settings.

    \begin{figure}[ht]
        \centering
        \begin{subfigure}[b]{0.32\textwidth}
            \includegraphics[width=\linewidth]{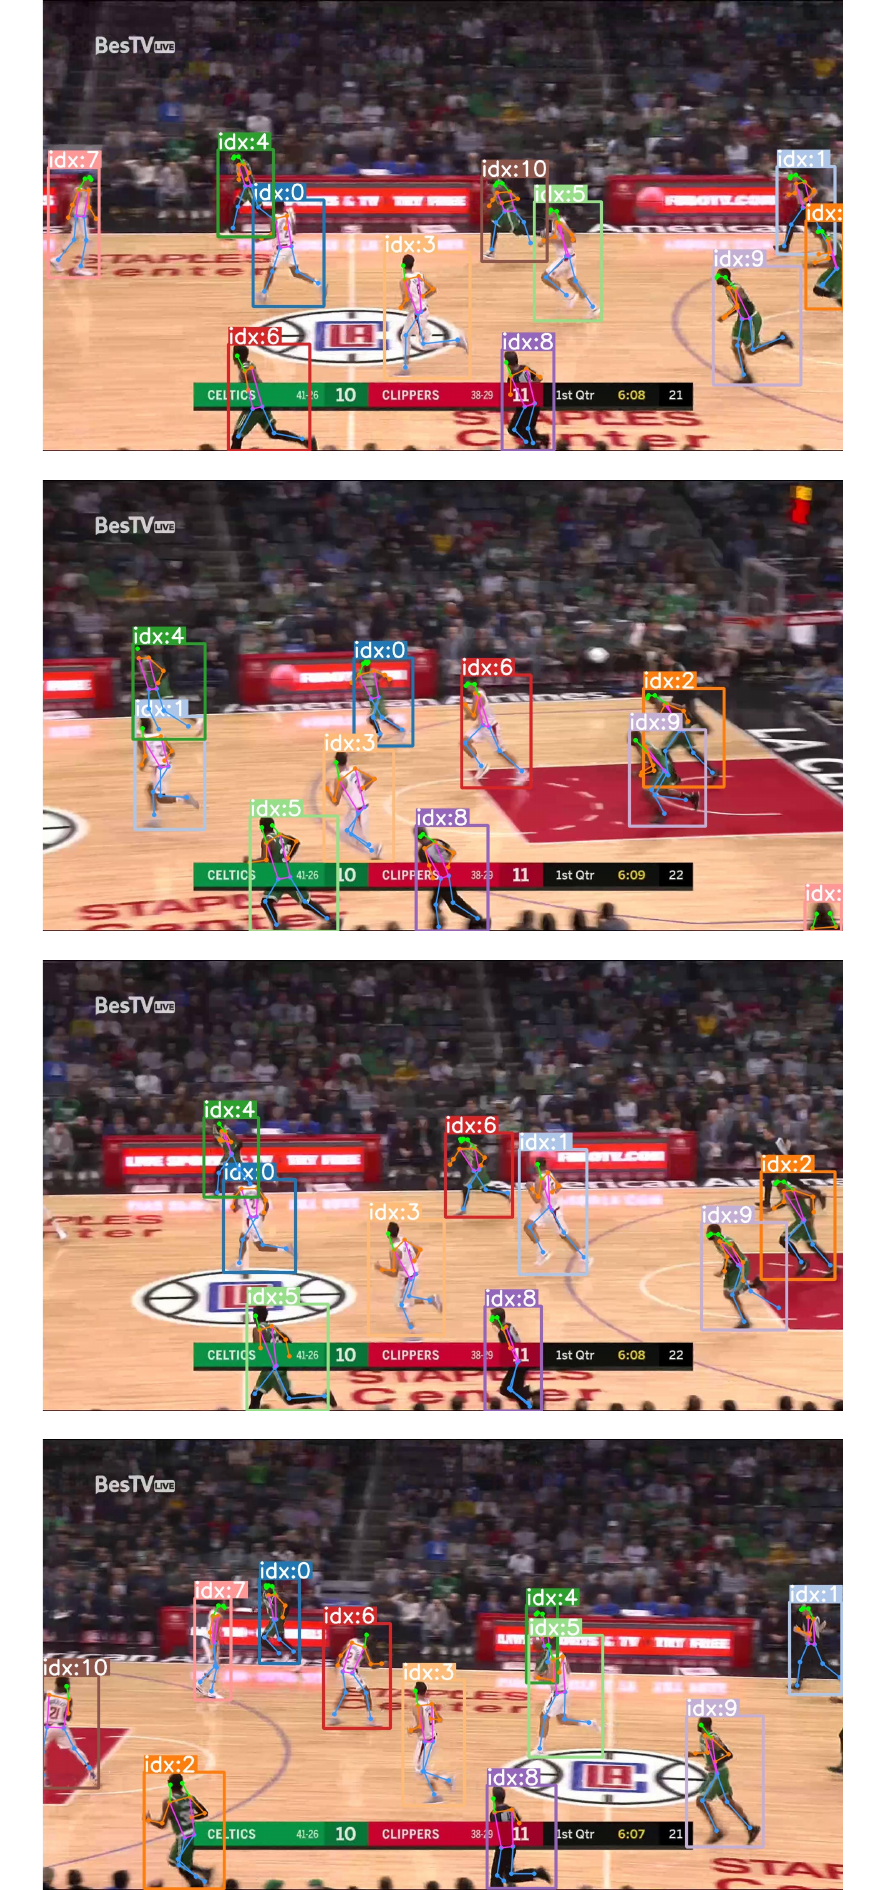}
            \caption{NBA}
            \label{fig:vis-a}
        \end{subfigure}
        \hfill
        \begin{subfigure}[b]{0.32\textwidth}
            \includegraphics[width=\linewidth]{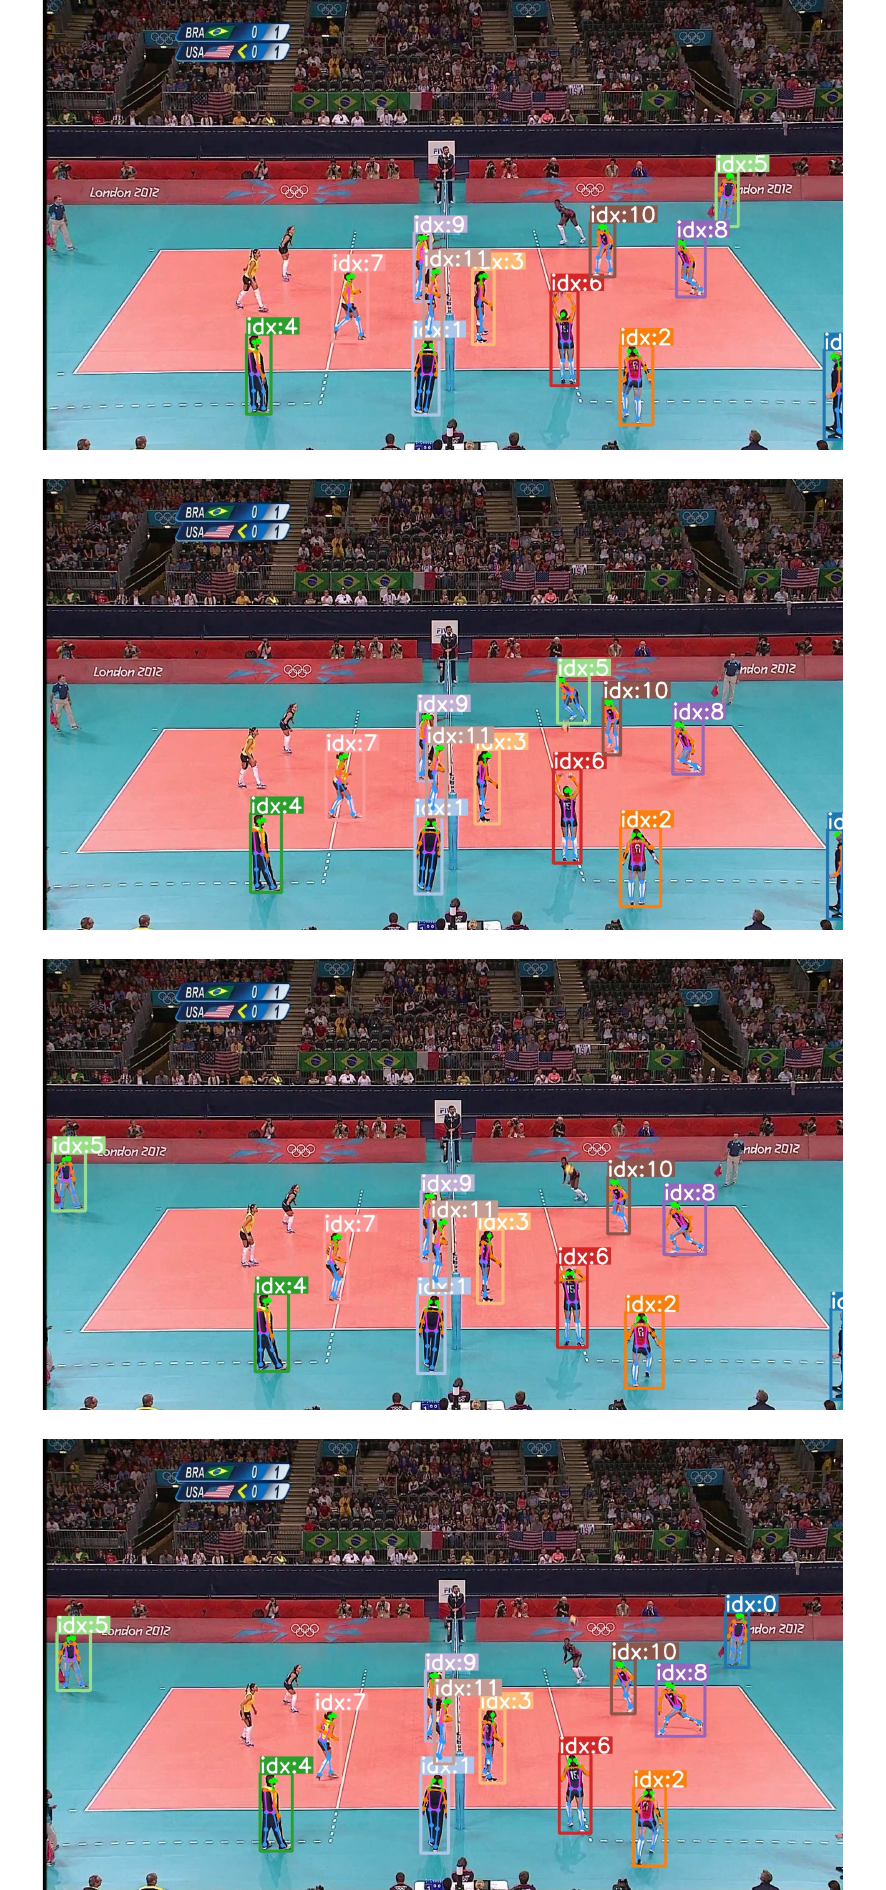}
            \caption{Volleyball Weak Supervised}
            \label{fig:vis-b}
        \end{subfigure}
        \hfill
        \begin{subfigure}[b]{0.32\textwidth}
            \includegraphics[width=\linewidth]{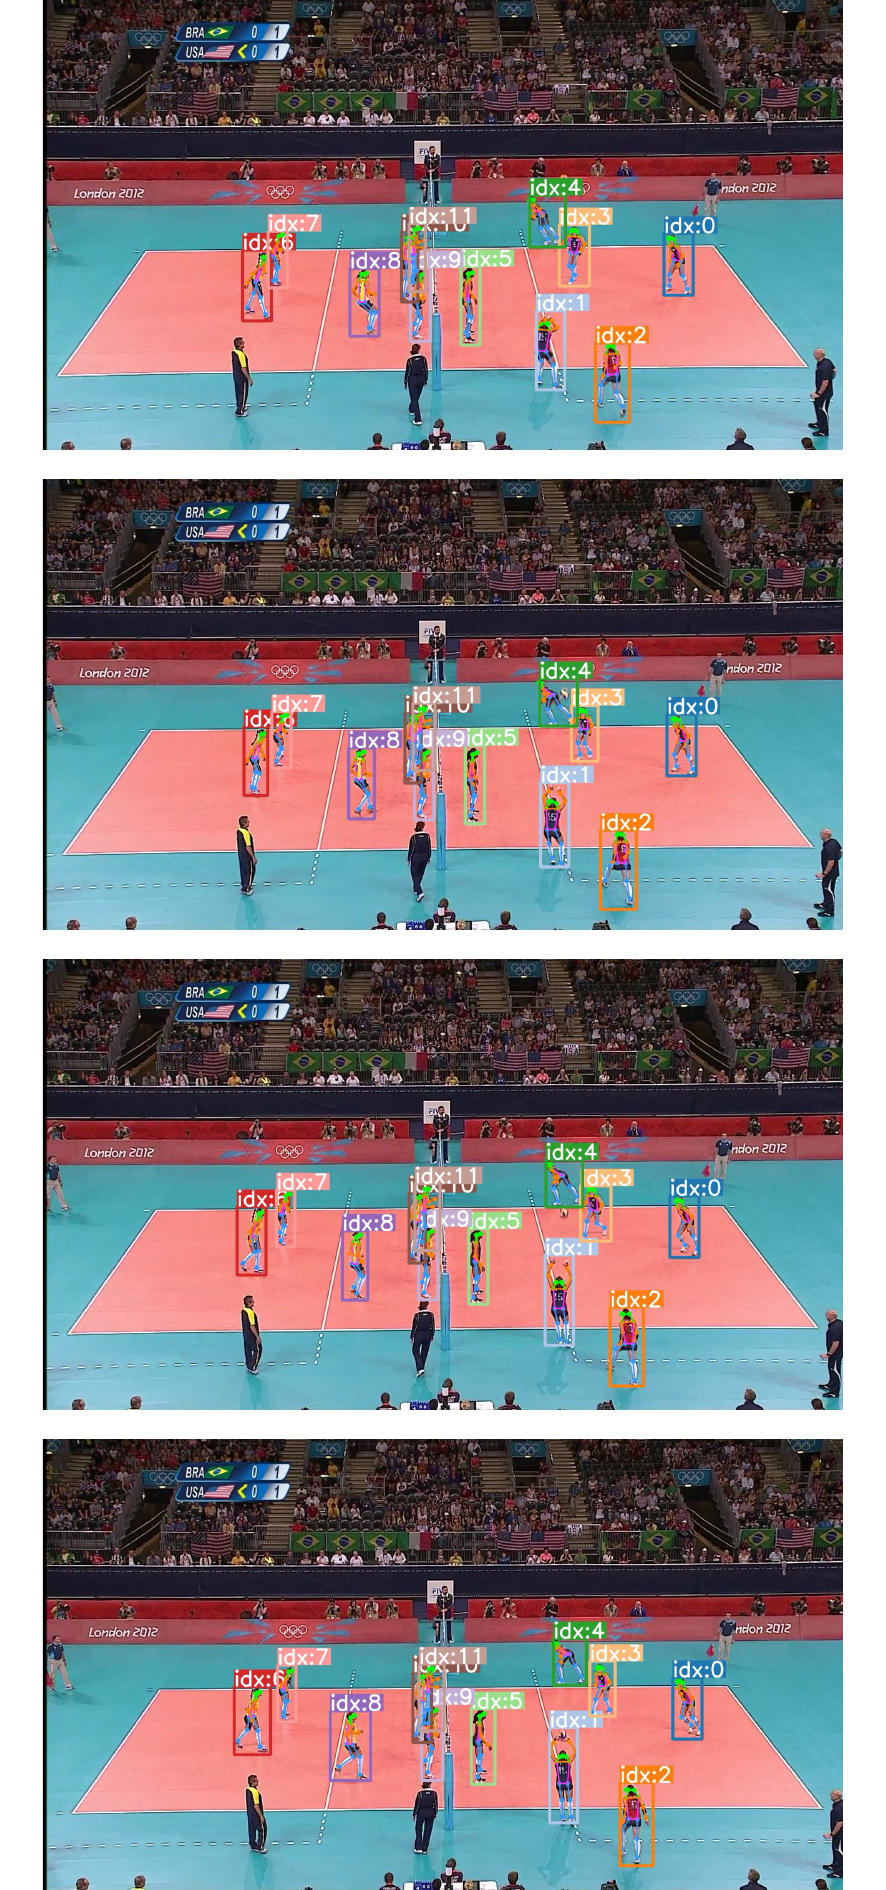}
            \caption{Volleyball Fully Supervised}
            \label{fig:vis-c}
        \end{subfigure}
        
        \caption{The extracted skeletons of the Volleyball Fully Supervised (with GT bounding boxes), Volleyball Weakly Supervised, and NBA datasets.}
        \label{fig:suppl-vis}
    \end{figure}

    \Cref{fig:suppl-vis} shows the visualization of the skeletal data used in our experiments. \Cref{fig:vis-a} illustrates the skeletons extracted from the NBA dataset during instances of high-speed camera movement. Although most actors can still be captured, the tracking results are not entirely satisfactory. \Cref{fig:vis-b} shows the results of extracting skeletons without using the ground truth individual detection. When compared with \cref{fig:vis-c} which uses the ground truth boxes, errors in detecting and selecting key roles are more likely to occur.

\begin{figure}[htp]
    \centering
    \begin{subfigure}[b]{0.4\linewidth}
        \includegraphics[width=\linewidth]{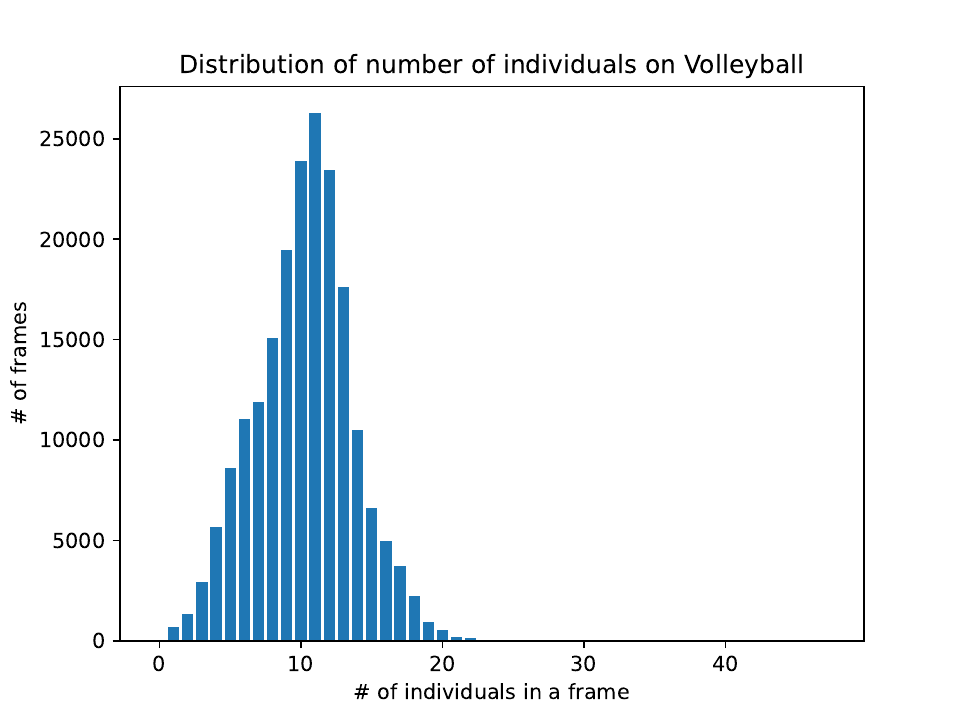}
        \caption{\#people on Volleyball}
        \label{fig:num-a}
    \end{subfigure}
    % \hfill
    \begin{subfigure}[b]{0.4\linewidth}
        \includegraphics[width=\linewidth]{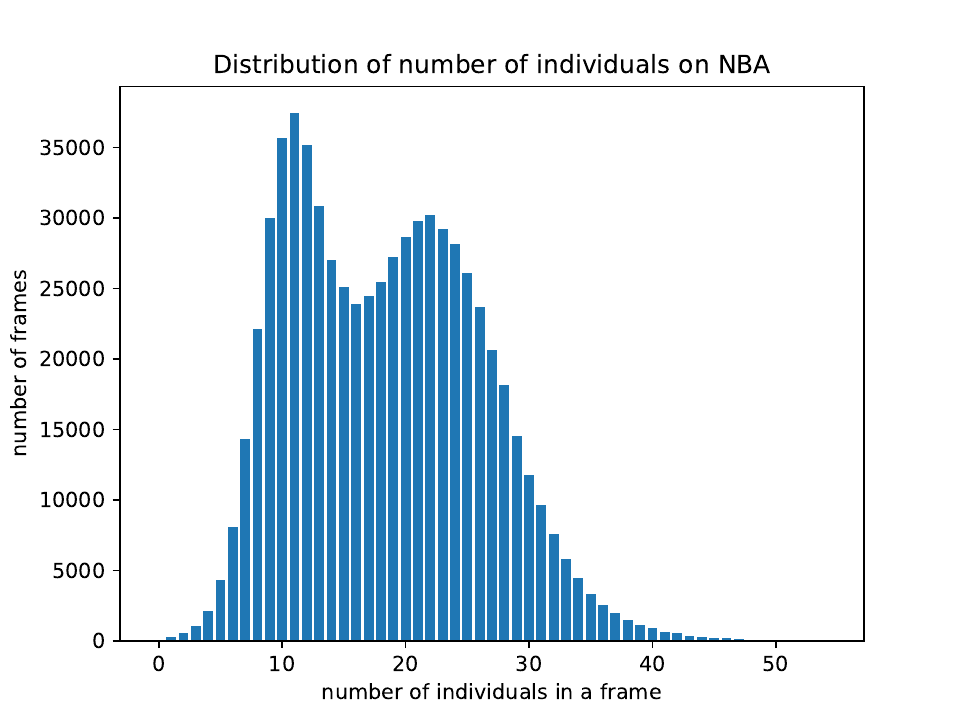}
        \caption{\#people on NBA}
        \label{fig:num-b}
    \end{subfigure}

    \begin{subfigure}[b]{0.4\linewidth}
        \includegraphics[width=\linewidth]{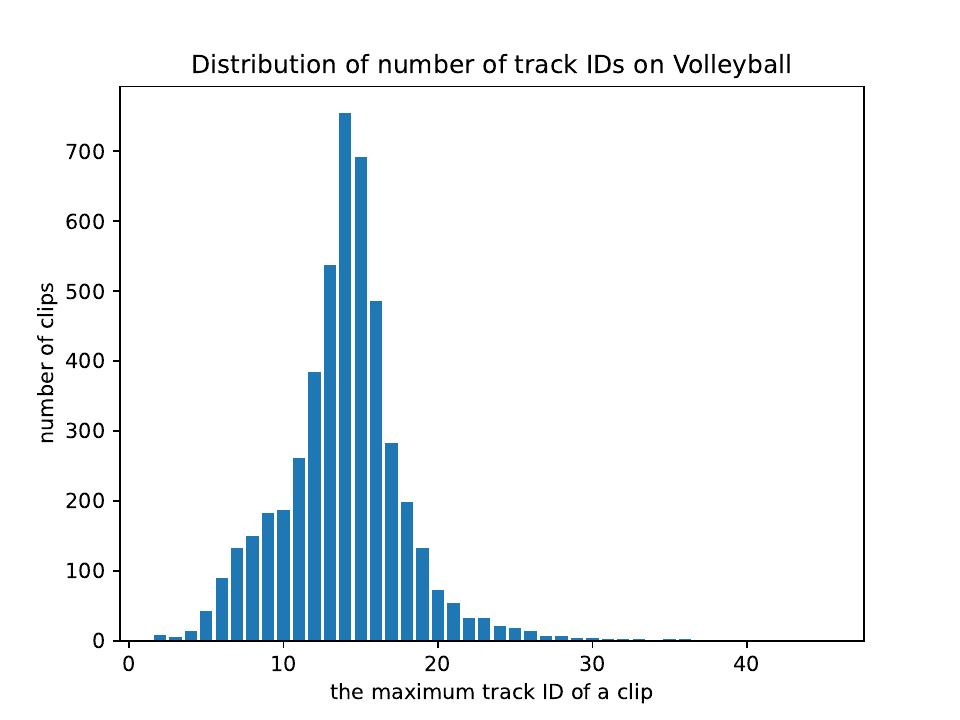}
        \caption{\#track IDs on Volleyball}
        \label{fig:num-c}
    \end{subfigure}
    % \hfill
    \begin{subfigure}[b]{0.4\linewidth}
        \includegraphics[width=\linewidth]{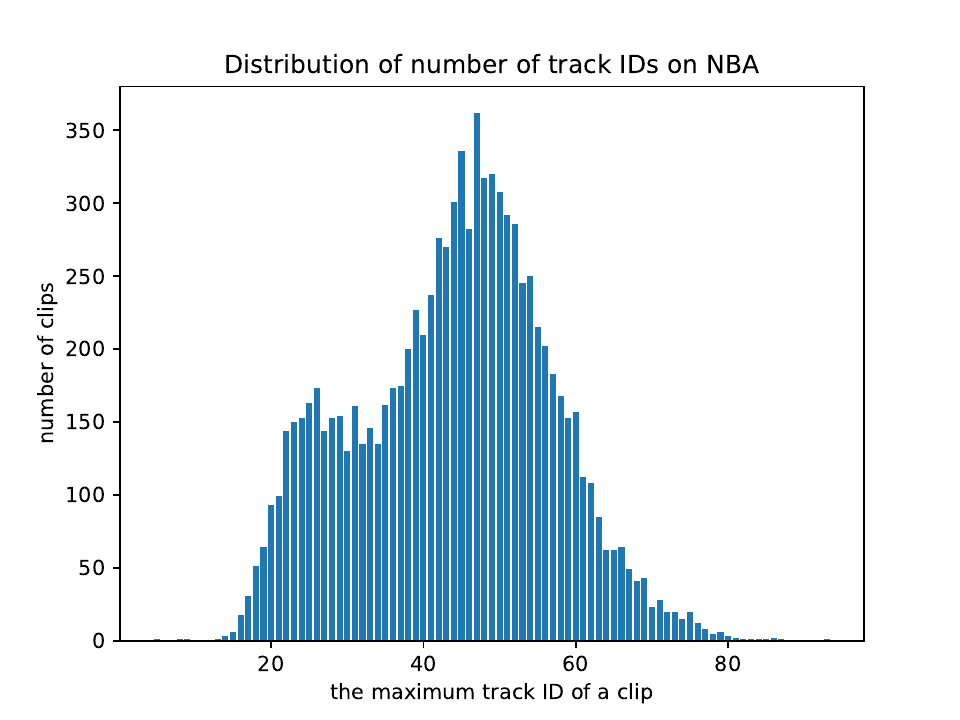}
        \caption{\#track IDs on NBA}
        \label{fig:num-d}
    \end{subfigure}

    \begin{subfigure}[b]{0.4\linewidth}
        \includegraphics[width=\linewidth]{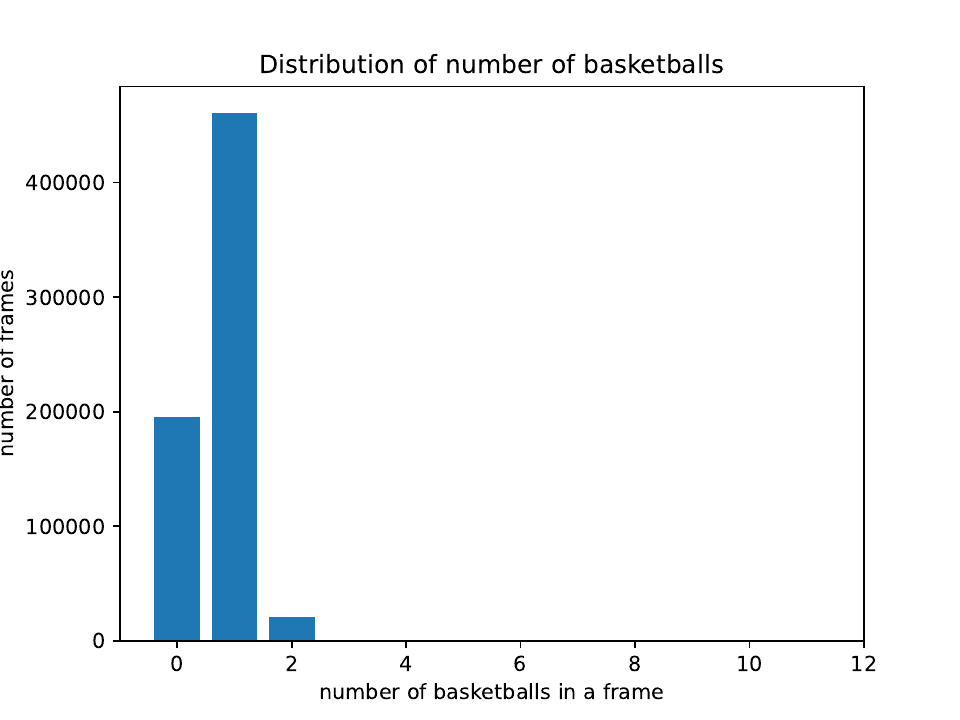}
        \caption{\#basketballs on NBA}
        \label{fig:num-e}
    \end{subfigure}
    % \hfill
    \begin{subfigure}[b]{0.4\linewidth}
        \includegraphics[width=\linewidth]{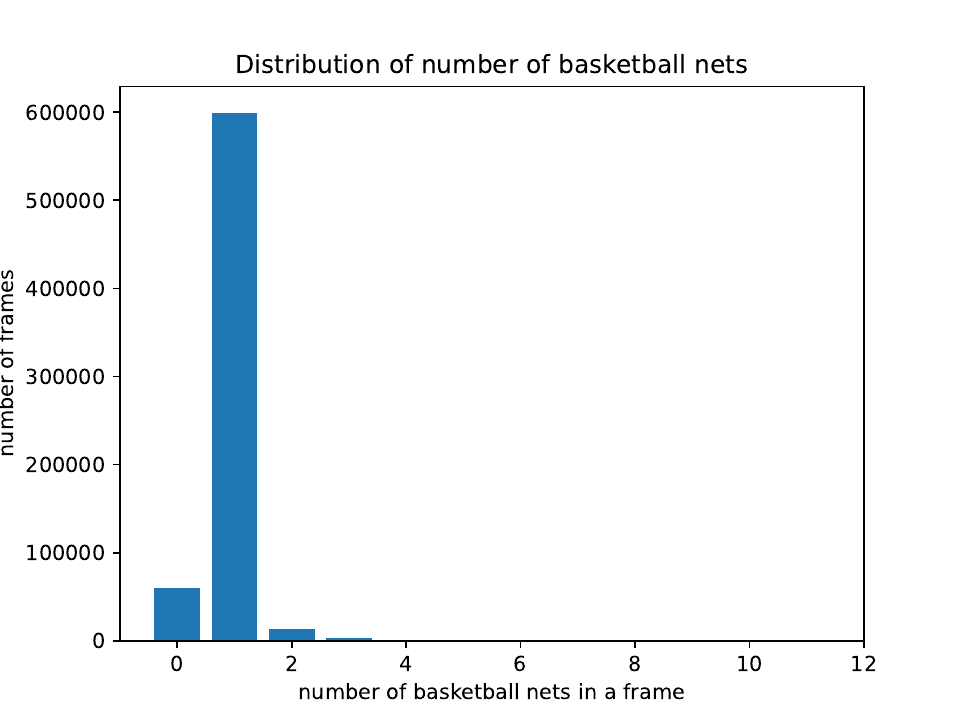}
        \caption{\#basketball nets on NBA}
        \label{fig:num-f}
    \end{subfigure}
    \caption{The distribution of the number of detected people in each frame, the number of track IDs in each clip, and the number of detected objects in each frame.}
    \label{fig:num-person}
\end{figure}

\begin{figure}
    \centering
    \includegraphics[width=0.5\linewidth]{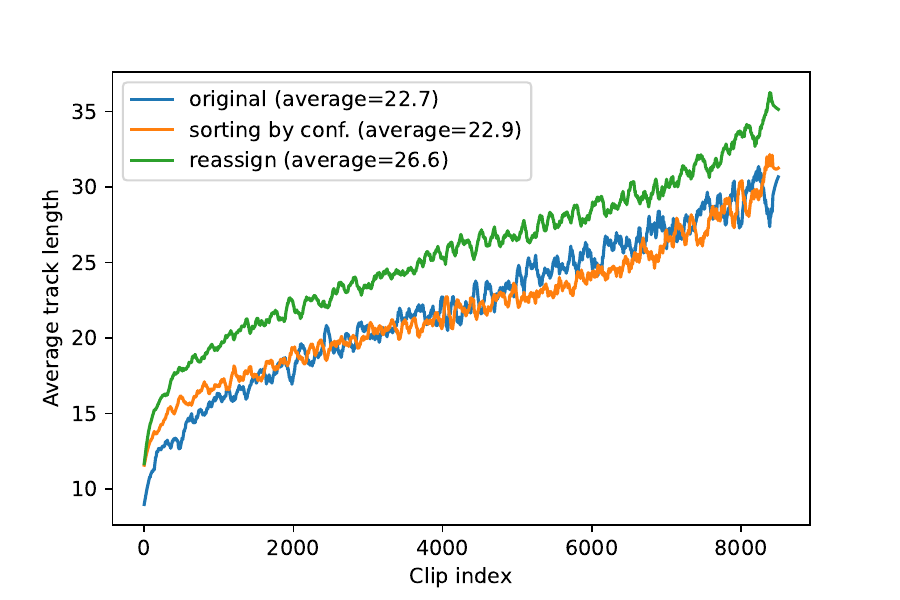}
    \caption{Comparison of the averaged track length per clip for the estimated skeletons from NBA dataset using different processing strategies, including the original estimation, sorting by confidence, and our proposed reassignment strategy.}
    \label{fig:track_len}
\end{figure}

    In \cref{fig:num-a,fig:num-b}, we illustrate the distribution of the number of individuals extracted in each frame from the Volleyball and NBA datasets. The number of individuals peaks at around 12 but frequently exceeds 20 in many frames. \Cref{fig:num-c,fig:num-d} present the number of track IDs detected by the tracker in each clip, revealing that the majority of clips contain more than 12 track IDs. These findings underscore the necessity of adopting a reassignment strategy to accurately track important individuals across frames.

    For the NBA dataset, the keypoints of basketball and basketball net are extracted using the YOLOV8x model. We initialize YOLOV8x with pre-trained weights and fine-tune for 50 epochs on the custom dataset. \Cref{fig:num-e,fig:num-f} present the number of basketball nets and basketballs detected in each frame. It can be observed that basketballs and basketball nets are detected in approximately 75\% of the frames and 90\% of the frames, respectively.

    \noindent
    \textbf{Backbone Efficiency Comparison.} \Cref{tab:backbone} compares the FLOPs for RGB backbones used by prior works and YOLOv8x. The results indicate that YOLOv8x is more efficient than backbones such as VGG-16 and VGG-19. It should be noted that the task of skeleton-based action recognition only uses an off-the-shelf pose backbone for keypoint extraction, which occurs once during dataset preparation. In offline scenarios, the efficiency of the pose backbone is not a critical factor in the overall efficiency. Therefore, larger pose estimators are acceptable when producing skeleton data from a video dataset. For online usage, more efficient real-time pose estimators can be applied to reduce computational costs and latency.

\begin{table}[tb]
    \centering
    \caption{Efficiency Comparison of RGB and pose backbones in FLOPs, $[T, H, W] = [1, 720, 1280]$.}
    \label{tab:backbone}
    \begin{tabular}{ccccc}
        \toprule
        YOLOv8x & VGG-16 & VGG-19 & Inception-v3 & ResNet-18 \\
        \midrule
        258G & 282G & 358G & 66G & 33.7G \\ 
        \bottomrule
    \end{tabular}
\end{table}

\subsection{Reassignment Strategy}
\label{sec:supp-ab}

    As illustrated in~\cref{fig:num-b,fig:num-d}, for the NBA dataset, about 23 people are detected in each frame, while the tracker produces an average of 50 track IDs per clip.
    These results indicate that issues such as missed detection and lost tracks occur frequently. Therefore, we propose a reassignment strategy to mitigated the inconsistency issues.
    
    In addition to the results presented in \cref{tab:detection}, we investigate the influence of different processing strategies on the average track length per video clip. \Cref{fig:track_len} compares the average tracking length per clip for the estimated skeletons from the NBA dataset using different processing strategies. These strategies include (1) the original estimation results, (2) selecting people with maximum confidences, and (3) the proposed reassignment strategy.
    The curve in \cref{fig:track_len} is produced by sorting by the mean track length of three strategies and smoothed using Savitzky–Golay filter.
    The reassignment strategy brings a steady improvement in the average tracking length (72 frames/clip) from 22.7 to 26.6 and brings $\sim$1.3\% improvement in accuracy compared to simply picking by maximum confidence.

    \noindent
    \textbf{Pose Estimation, Tracking and Reassignment.} \Cref{tab:detection} summarizes the performance of our method using skeletons extracted by different methods~\cite{sun2019hrnet, fang2023alphapose} which are widely used in skeleton-based action recognition~\cite{li2021groupformer, zhou2022composer, duan2022revisiting}. The results indicate that our proposed reassignment strategy coupled with a tracking algorithm leads to a marked improvement in performance.

\begin{table}[t]
    \centering
    \caption{Comparison of our method with only human skeleton data obtained by widely-used pose estimation and tracking algorithms in MCA (\%) on NBA dataset}
    \label{tab:detection}
    \begin{tabular}{llc|c}
        \toprule
            Pose Estimator & ReID Tracker  & Reassign & MCA \\ % & Pose+Ball \\ 
        \midrule
            HRNet~\cite{sun2019hrnet} & no tracking & & 64.60 \\ % & 72.80 \\
        \midrule
            \multirow{2}*{AlphaPose~\cite{fang2023alphapose}} & no tracking & & 64.92 \\
            ~ & JDE~\cite{wang2020jde} & $\checkmark$ & 65.57 \\ % & 73.11 \\
        \midrule
            \multirow{3}*{YOLOv8x~\cite{jocher2023yolov8}} & no tracking & & 67.02 \\ % & 73.71 \\ 
            % ~ & ByteTrack~\cite{zhang2022bytetrack} & $\checkmark$ & 64.82 & 73.84 \\
            ~ & BoT-SORT~\cite{aharon2022botsort} & ~ & 67.95 \\ % & 74.18 \\
            ~ & BoT-SORT~\cite{aharon2022botsort} (Ours) & $\checkmark$ & \textbf{69.21} \\ % & \textbf{75.56} \\
        \bottomrule
    \end{tabular}
\end{table}

\section{Data Pre-processing of Multiple Inputs}
\label{sec:supp-b}

    In this paper, we build upon previous studies in skeleton-based human action recognition~\cite{shi2019-2sagcn,liu2020disentangling,chen2021ctrgcn,song2023effgcn}, developing four types of input features: 1) joint coordinates, 2) bone vectors, 3) joint motion features, and 4) bone motion features.

    Suppose the original 2D/3D coordinates of a group activity sequence is $\mathcal{X}\in\mathbb{R}^{T\times MN\times C}$, where $T$, $M$, $N$, $C$ denote the number of frames, number of people, number of joints and input coordinates, respectively. For the Volleyball Fully Supervised, we adopt $C=2$ to indicate the two-dimension keypoint coordinates. For the NBA and Volleyball Weakly Supervised datasets, we use $C=3$ to represent the set $\{x,y,v\}$, where $v$ denotes the visibility prediction from the pose backbone.

    The input of joint coordinates is the concatenation of absolute locations $\mathcal{X}$ and relative locations to the body center $\mathcal{X}_{relative}$, where
    \begin{equation}
        \mathcal{X}_{relative}[:,i,:] = \mathcal{X}[:,i,:] - \mathcal{X}[:,{center}_m,:],
    \end{equation}
    $i=\{1,2,\dots,MN\}$, and ${center}_m$ represents the index of the center joint of person $m$. The input of bone features is obtained by concatenating the bone vectors and their angles relative to the coordinate axes.
    \begin{equation}
    \label{eq:bone}
    \begin{split}
        \mathcal{X}_{bone}[:,i,:] = \mathcal{X}[:,i,:] - \mathcal{X}[:,i_{adj},:], \\
        \mathcal{X}_{angle}[:,i,c] = \arccos{
        \frac{\mathcal{X}_{bone}[:,i:c]}{\sqrt{||\mathcal{X}_{bone}[:,i,:] ||^2}}}.
    \end{split}
    \end{equation}
    In \cref{eq:bone}, $i_{adj}$ denotes the adjacent node of joint $i$, and $c={1,2}$ denotes the 2D coordinates and $c={1,2,3}$ denotes the 3D coordinates.
    
    Furthermore, the joint motion features are the concatenation of the motion ${X}_{jm1}$ between consecutive frames and ${X}_{jm2}$ two-hop frames.
    \begin{equation}
    \begin{split}
    \label{eq:joint-motion}
        \mathcal{X}_{jm1}[t,:,:] = \mathcal{X}[t+1,:,:] - \mathcal{X}[t,:,:], \\ 
        \mathcal{X}_{jm2}[t,:,:] = \mathcal{X}[t+2,:,:] - \mathcal{X}[t,:,:].
    \end{split}
    \end{equation}
    In \cref{eq:joint-motion}, $t=\{1,2,\dots,T\}$. Similarly, the bone motion features are calculated by connecting the motion of bone features ${X}_{bm1}$ and ${X}_{bm2}$.
    \begin{equation}
    \begin{split}
        \mathcal{X}_{bm1}[t,:,:] = \mathcal{X}_{bone}[t+1,:,:] - \mathcal{X}_{bone}[t,:,:], \\ 
        \mathcal{X}_{bm2}[t,:,:] = \mathcal{X}_{bone}[t+2,:,:] - \mathcal{X}_{bone}[t,:,:].
    \end{split}
    \end{equation}

    Afterwards, these four features in $T\times MN\times 2C$ are feed into four separate input branches, respectively.

    % \begin{table}[t]
    %     \centering
    %     \caption{Comparison of different input data either with early fusion or with late fusion technique in MCA (\%) and FLOPs on the NBA dataset.}
    %     \label{tab:input}
    %     \begin{tabular}{c|cc}
    %     \toprule
    %     Input data   & FLOPs & MCA\\
    %     \midrule
    %     Joint (J) & \multirow{4}*{14.4G} & 73.74 \\
    %     Bone (B)  & ~                   & 74.25 \\
    %     Joint motion (JM) &  ~            & 64.31 \\
    %     Bone motion (BM) & ~             & 63.43 \\
    %     J + B  & 17.2G                       & 75.24 \\
    %     J + B + JM & 19.8G                   & 75.53 \\
    %     \textbf{J + B + JM + BM (ours)} & 22.3G  & 75.96 \\
    %     J + B (late fusion)    & 25.2G       & 77.13 \\
    %     J + B + JM (late fusion) & 37.8G     & 78.49 \\
    %     J + B + JM + BM (late fusion) & 50.4G & \textbf{78.68} \\
    %     \bottomrule
    %     \end{tabular}
    % \end{table}

    % \Cref{tab:input} presents the classification accuracy of our model with different input features when using either the early-fusion or late-fusion architecture. It can be observed that the late-fusion method achieves a higher MCA than the early-fusion methods, at the expense of increased computational costs.

\section{Detailed Comparison between Keypoint-based Methods}
\label{sec:supp-c}

In this section, we provide more detailed comparisons between our method and state-of-the-art keypoint-based methods on the Volleyball and NBA dataset. We also compare our method with GCNs in skeleton-based action recognition.

\begin{table}[t]
    \centering
    \caption{Comparisons with state-of-the-art (SOTA) methods that leverage only keypoint information on the Volleyball Dataset.}
    \label{tab:volleyball-keypoint}
    \begin{tabular}{lcccc}
    \toprule
    Method & Pose Backbone & Pose & Object & Acc. \\
    \midrule
    \multirow{2}*{GIRN~\cite{perez2022skeletonbased}} & \multirow{2}*{OpenPose} & \checkmark & & 88.4 \\ 
    ~ & ~ & \checkmark & \checkmark & 92.2 \\ 
    \midrule
    \multirow{2}*{AT~\cite{gavrilyuk2020actortransformers}} & \multirow{2}*{HRNet} & \checkmark & & 92.3 \\
    ~ & ~ & \checkmark & \checkmark & 92.8 \\
    \midrule
    \multirow{2}*{POGARS~\cite{thilakarathne2022pose}} & \multirow{2}*{Hourglass} & \checkmark & & 93.2 \\
    ~ & ~ & \checkmark & \checkmark & 93.9 \\
    \midrule
    \multirow{2}*{COMPOSER~\cite{zhou2022composer}} & \multirow{2}*{HRNet} & \checkmark & & 93.7 \\
    ~ & ~ & \checkmark & \checkmark & 94.6 \\
    \midrule
    SkeleTR~\cite{duan2023skeletr} & HRNet & \checkmark & & 94.4 \\
    \midrule
    \multirow{2}*{MP-GCN (Ours)} & \multirow{2}*{HRNet} & \checkmark & & \underline{95.2} \\
    ~ & ~ & \checkmark & \checkmark & \textbf{95.5} \\
    \bottomrule
    \end{tabular}
\end{table}

\Cref{tab:volleyball-keypoint} presents the comparison of our method with state-of-the-art methods that leverage only keypoint information on the Volleyball dataset. With only human pose keypoints, our method achieves higher accuracy than others with even object keypoints. This result demonstrates the effectiveness of our proposed multi-person graph structure. When incorporating object keypoints, our method achieves the highest accuracy of 95.5\% among all keypoint-based methods.

\begin{table}[t]
    \centering
    \caption{SOTA Comparison with GCNs on Volleyball and NBA datasets.}
    \label{tab:compare-gcns}
    \resizebox{\linewidth}{!}{
    \begin{tabular}{lc|ccc|ccc}
    \toprule
    \multirow{2}*{Model} & \multirow{2}*{\#Param.} & \multicolumn{3}{c|}{Volleyball} & \multicolumn{3}{c}{NBA} \\
    ~ & ~ & FLOPs & Pose & Pose+Obj & FLOPs & Pose & Pose+Obj \\
    \midrule
    ST-GCN~\cite{yan2018stgcn} 
        & 3.08M & 4.9G & 89.15 & 91.30 & 18.6G & 52.00 & 66.8 \\
    MS-G3D~\cite{liu2020disentangling}(2-ensemble) 
        & 6.01M & 18.9G & 93.19 & 94.17 & 68.0G & 66.34 & 76.23 \\
    CTR-GCN~\cite{chen2021ctrgcn}(4-ensemble) 
        & 5.71M & 11.9G & 93.56 & 94.54 & 39.0G & 70.09 & 76.29 \\
    HD-GCN~\cite{lee2023hdgcn}(6-ensemble) 
        & 7.81M & 13.6G & 93.71 & 94.91 & 45.2G & 69.83 & \underline{77.39} \\
    \midrule
    MP-GCN (Ours)
        & 4.40M & 4.2G & \underline{95.21} & \underline{95.54} & 22.3G & \textbf{72.94} & 75.96 \\
    MP-GCN (4-ensemble)
        & 11.58M & 13.20G & \textbf{95.23} & \textbf{95.67} & 48.6G & \underline{72.77} & \textbf{78.68} \\
    \bottomrule
    \end{tabular}
    }
\end{table}

\Cref{tab:compare-gcns} presents the comparison of our method with GCNs in skeleton-based human action recognition. Each GCN adopts its original ensemble technique and single-person graph scale but includes extra ball and basketball net keypoints. All methods are evaluated using the same skeleton and object data as ours. Our method achieves the highest performance on both datasets when using the same emsemble technique. Simply transferring these methods to group activity recognition does not obtain the greatest performance, since they are specifically designed and tuned for single-person action recognition. 



\section{Additional Qualitative Results}
\label{sec:supp-d}

We provide additional quantitative and qualitative results that are not included in the main paper due to page constraints.

\begin{figure}[tb]
    \centering
    \begin{subfigure}[b]{0.46\textwidth}
        \includegraphics[width=\linewidth]{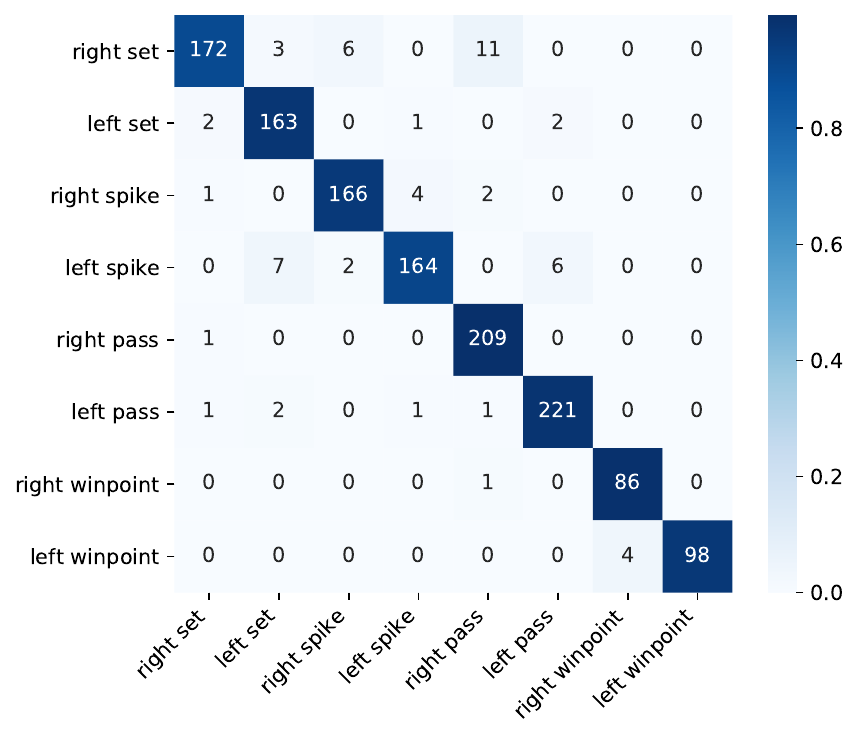}
        \caption{Volleyball Fully Supervised}
        \label{fig:cm-a}
    \end{subfigure}
    \hfill
    \begin{subfigure}[b]{0.46\textwidth}
        \includegraphics[width=\linewidth]{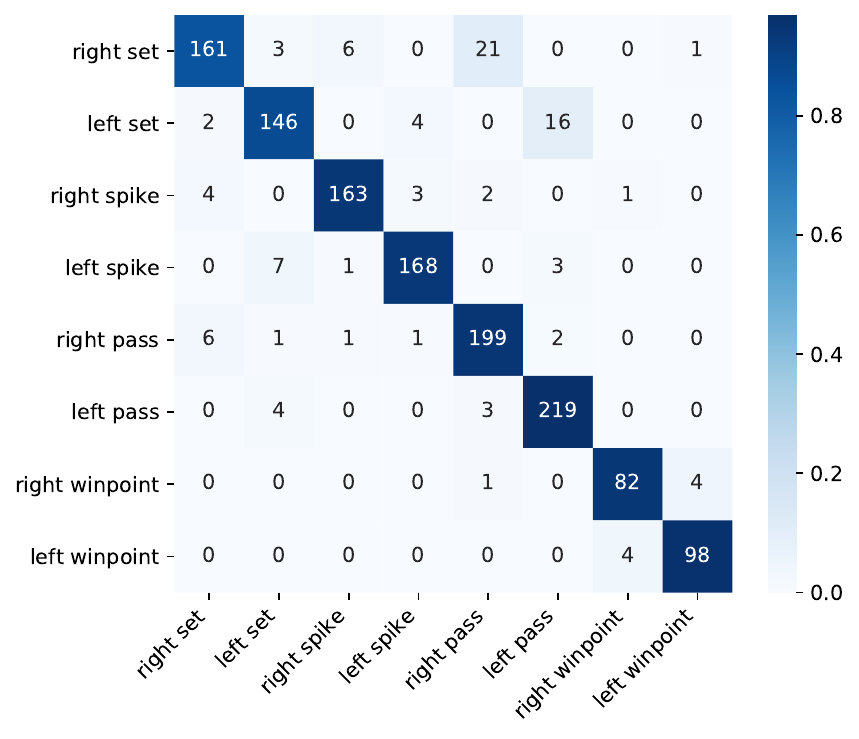}
        \caption{Volleyball Weakly Supervised}
        \label{fig:cm-b}
    \end{subfigure}
    \hfill
    \begin{subfigure}[b]{0.7\textwidth}
        \includegraphics[width=\linewidth]{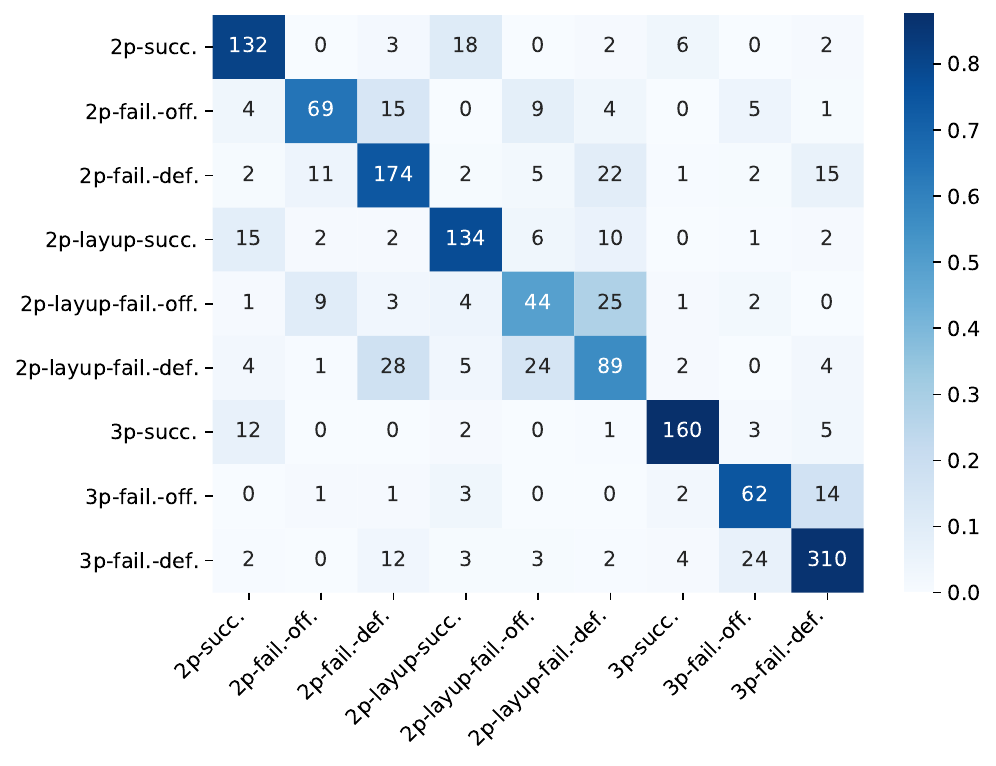}
        \caption{NBA}
        \label{fig:cm-c}
    \end{subfigure}
    
    \caption{The confusion matrices on Volleyball Fully Supervised, Volleyball Weakly Supervised, and NBA datasets.}
    \label{fig:cm}
\end{figure}

\begin{figure}[tb]
    \centering
    \includegraphics[width=0.95\textwidth]{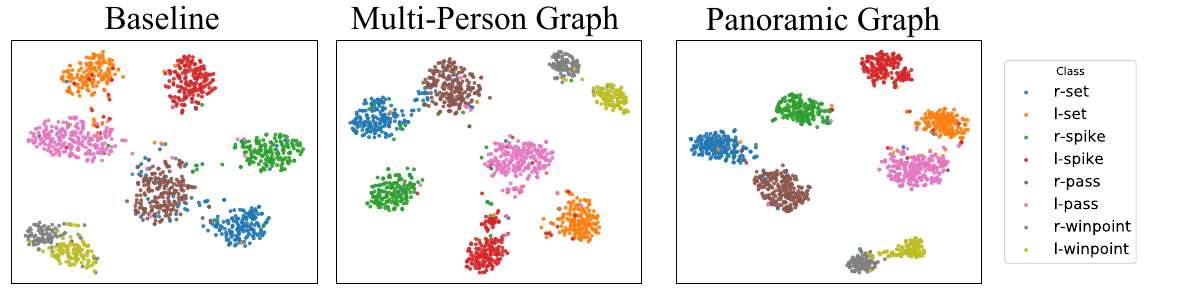}
    \caption{$t$-SNE feature embedding visualization on the Volleyball dataset by different graph structure.}
    \label{fig:tsne-volleyball}
\end{figure}

\textbf{Comfusion Matrix}. \Cref{fig:cm} presents the confusion matrix on Volleyball Fully Supervised, Volleyball Weakly Supervised and NBA dataset. As shown in~\cref{fig:cm-a}, a majority samples are classified correctly, with exceptions for cases such as \textit{right set} and \textit{right pass}. For the Volleyball dataset in weakly supervised setting (\Cref{fig:cm-b}), the overall accuracy decreases, primarily due to the confusion of \textit{left set}-\textit{left pass} and \textit{right set}-\textit{right pass}. This result may be attributed to the absence of ground-truth detection boxes, leading to missed detection and inaccurate tracking of key actors. For the NBA dataset (\Cref{fig:cm-c}), the most confusing cases are \textit{layup-fail.-off.}-\textit{layup-fail.-def.}. These two types of actions can only be differentiated by whether the offensive or defensive team gets the rebound after the ball is thrown.

\textbf{t-SNE Visualization}. \Cref{fig:tsne-volleyball} displays the $t$-SNE visualization of different graph structures on the Volleyball Fully Supervised dataset. It is evident that the proposed multi-person-object graph facilitates a clear separation of each class. 

\section{Additional Ablation Studies}
\label{sec:supp-e}

In this section, we present extra ablation studies that are not included in the main paper due to page limit, including experiments on network modules, inter-body graph topologies, and input dimensions.

\Cref{tab:module} illustrates the impact of different input branches and modules within the basic block. For the model that without SGC, we utilize a graph with only self-link edges as a substitute. For the model without TCN, we replace the multi-scale temporal convolution layer with a standard $5\times1$ temporal convolution. These results demonstrate that each component of the basic block substantially contributes to the model's recognition capabilities.

\begin{table}[t]
    \hfill
    % \begin{minipage}[t]{0.43\textwidth}
    \centering
    \caption{Comparison of different network modules in terms of MCA on Volleyball Weakly Supervised and NBA dataset.}
    \label{tab:module}
    % \resizebox{\linewidth}{!}{
    \begin{tabular}{ll|cc}
        \toprule
            Module & Model Config & Volleyball & NBA \\
        \midrule
            \multirow{3}*{Input Branch} & J & 87.81  & 73.74 \\
            & J+B   & 91.47 & 75.24 \\
            & J+B+JM & 91.92 & 75.53 \\
        \midrule
            \multirow{3}*{Basic Block} & w/o SGC & 90.25 & 72.87 \\
            & w/o TCN   & 92.00 & 72.29 \\
            % spatial labeling & 92.1 & 73.28\\ 
            & w/o Attention    & 91.35 & 73.32 \\
        \midrule
        Ours &  J+B+JM+BM & \textbf{92.77} & \textbf{75.96} \\
        \bottomrule
    \end{tabular}
        % }
    % \end{minipage}
\end{table}

\Cref{tab:inter-body} shows the impact of various inter-body links on the Volleyball Fully Supervised dataset. To maintain sufficient sparsity in the inter-body connections, we experiment with several connection strategies based on body centers and object keypoints. These strategies include: (1) None: No inter-body connections; (2) Fully-Connected: A fully connected graph within $M$ body centers. (3) Linear: A linear graph with sequential connections (4) Pairwise: Connections established between pairs of individuals. The experimental results indicate that the pairwise connection strategy  achieves higher accuracy. Additionally, we observed that it brings a more stable training process. In our future research, we plan to explore a broader range of topological structures for inter-body connections to potentially enhance performance further.

In \cref{tab:dim}, we compare the performance between 2-dimensional input ($\{x,y\}$) and 3-dimensional input ($\{x,y,v\}$) with visibility evaluation. For both types of input data, the addition of a visibility input provides more information and improves the MCA by over 1\%. 

\begin{table}[t]
    \begin{minipage}[t]{0.38\linewidth}
        \centering
        \caption{Comparison of different inter-body links in MCA (\%) on the Volleyball dataset.}
        \label{tab:inter-body}
        \begin{tabular}{l|c}
        \toprule
        Inter-body Graph & MCA\\
        \midrule
        None  & 95.21 \\ 
        Fully-Connected & 94.84 \\
        Linear & 95.14 \\
        Pairwise (Ours) & \textbf{95.54} \\
        \bottomrule
        \end{tabular}

    \end{minipage}
    \hfill
    \begin{minipage}[t]{0.6\linewidth}
        \centering
        \caption{Comparison of different input dimensions in MCA (\%) on the NBA dataset.}
        \label{tab:dim}
        \begin{tabular}{ll|c}
        \toprule
        Dimension & Input data & MCA \\
        \midrule
        \multirow{2}*{2-$\{x,y\}$} & pose & 68.03 \\
        ~     & pose+object & 74.48 \\
        \midrule
        \multirow{2}*{3-$\{x,y,v\}$} & pose & 69.21 \\
        ~     & pose+object & \textbf{75.96} \\ 
        \bottomrule
        \end{tabular}

    \end{minipage}
\end{table}
